# Supplementary material for: Relaxing Concurrent Data-structure Semantics for Increasing Performance: A Multi-structure 2D Design Framework
Source: arXiv:1906.07105 source file (2023-01-21)
Supplement: Supplementary file 1 [file appendix.tex]

\section*{Appendix}%
